# Supplementary material for: A Deep Learning Strategy for Vehicular Floating Content Management
Source: arXiv:1811.11249 source file (2018-10-24)
Supplement: Supplementary file 1 [file appendix.tex]

\appendix

\section{Spare material}
%%%%application level
%\subsection{Application Level: The high-dimensional issue}  
%The approach used is versatile, it can be used for a variety of applications such as advertisements, rerouting, and emergency. 
%%%%application which we are aim to
%One among others, which to the best of our knowledge, no studies on FC face it, is traffic congestion. Indeed, the 2015 Urban Mobility Report indicates, in the “invoice” for the cost of extra time and fuel in the 471 U.S. urban areas \cite{urban_}, that congestion causes 6.9 billion hours of extra time, 3.1 billion gallons of wasted fuel corresponding to a congestion cost of 160 billion dollars. 
%Therefore, understanding how the message should be spread to decrease the ripples throughout large-scale network is vital to pinpoint traffic bottlenecks for congestion mitigation.

%%%high-dimensional space issue 
%The increasing availability of data network makes possible, to examine traffic flows on a large-scale roadway network, and observe the evolution of congestion on network, through data mining techniques. However, due to the tremendous traffic sensors growth on the existing roadway networks, which generate a huge amount of data, and the thousands of links with changing traffic condition over time, this issue is high-dimensional space where congestion changes temporally and spatially. 
%%%why machine learning is a good candidate 
%Machine learning theory can address this issue, in particular via deep learning technique which holds great promise in learning in high-dimensional features with tremendous data.

\subsection{Floating Content implementation}
FC is an infrastructure-less communication scheme which limited content exchange and storage in a geographical area called Anchor Zone (AZ). The AZ can have an arbitrary shape where within opportunistic communications between nodes take place. Application-based, the first content (seed) can be generated by a node or by an infrastructure if required. Whereas, the message is erased when its keeper exits the AZ. Previous works on FC, assume that the AZ is located and fixed at a specific area. In this work, we use infrastructure supports to reshape and relocate one or more AZs, based on the end-to-end goals of the application. As result of its distributed approach, FC is suitable for a variety of fields such as VANETs and IoT. From this last network, via device-to-device communication (D2D), is possible to find an implementation of FC. D2D communication can occur on the cellular spectrum or unlicensed spectrum~\cite{surv_D2D}. On the cellular spectrum, the bandwidth is partitioned between D2D and Cellular communication (i.e., overlay inband). In this scenario is possible to implement FC paradigm~\cite{alloc_D2D}. On the one hand, allocating D2D bandwidth when the node is within the AZ, on the other hand, deallocating when the node is out of it.    
% \subsection{for the next paper}
% we consider the case in which FC is used for traffic congestion warnings. We assume a given model for how nodes mobility changes according to information about traffic congestion. We set our goal as to limit the increase in average travel time due to congestion below a given percentage. We propose an approach based on ML which adapts in real time FC parameters to mobility, in a way which achieves the target performance while minimizing the overall cost (modeled through a given cost function) during the whole duration of the congestion period. 

% % %%%%mobility changes 
% % In particular, we take into account a city map where an accident, in a specific location, occurs. Considering that vehicles are event-based (i.e., changes their mobility on content received), our idea is to inform the users, via V2V communication, about the traffic congestion in order to avoid it.
% % %%%%granularity
% % On the one hand, the congestion level is our performance parameter. On the other hand, the AZ area represents the cost (e.g., in terms of bandwidth and energy). In this work, we reduce the AZ granularity in terms of roadway. The aim is to find the most efficient AZ set subject to the minimum traffic congestion level concerning the minimum resources usage.
% % %%%time-based
% % The AZ set (i.e., road enable for the communication) adapts to nodes mobility and performance parameters at each time. This time-based approach so, is suitable for short and long application-time.  


% \begin{defn}[Congestion]
% Given a link in $\textit{\textbf{l}}$, at time $t$ we consider the link congested if the average speed among the vehicles in it, is less than $20\ km/hour$ for more than $15$ seconds.    
% \end{defn}

% Note that the above definition includes most of the event where vehicle mobility changes such as car crash.

% When an event occurred, vehicles interested, start to broadcast the message till the issue is solved. In case of link congestion, when the interested road is not anymore blocked, the point is addressed.
% In particular, nodes involved in the congestion areas are the seeders, the message sources till the simulation ends. 

% Nodes assisting the event or informed vehicles, react according to an arbitrary rerouting model. 
% Additionally, probe vehicles have been recently implemented to provide real-time information on link travel times~\cite{agent}.
% Based on these different sources of traffic information, route distances and travel-times can be readily calculated~\cite{reroutecal}.

% As the final attempt, we aim to the congestion application. The goal is to inform vehicles to avoid the set of links congested. Therefore, in this application, nodes adapt their mobility based on the content received. 
% When the link is congested (i.e., the average speed at that time is below the given threshold), it has a cost. This cost, at time $t$, depends on the link node density ($V_c+V_{nc}$), contact density ($\lambda$), and nodes average speed ($\nu$). Analytically, 

% On the one hand, the more nodes are informed the higher is the probability of reducing the congestion area, i.e., vehicles involved in the congestion. On the other hand, the bigger the AZ, the higher costs (e.g., bandwidth used). 
% Moreover, note that configuration of $A$ at time $t$, involves the cost level at time $t$ but since the mobility has its dynamic, the congestion level, given $A^t$, will be measured at $t+1$. 

% \begin{problem}
% Given $P^t$,
% \begin{equation}
%   \minimize_{A^t}\quad k\sum_{i=1}^{N_{cong}}\frac{(V_c+V_{nc})_i}{\nu_i+1}+\sum_{i=1}^{N}A_i\frac{\lambda_i(V_c+V_{nc})_iTx_i}{t_{\lambda_i}},
% \end{equation}
% with $k\geq0$ as coefficient of the relative weight between the two cost components.
% \end{problem}

%\mah{Moreover, due to road grid restrictions, several nodes are may not able to avoid the congestion. Therefore, these nodes will congest other links, which will be considered as part of the initial sub-set of congested links.}

%\mah{Vehicles are equipped with IEEE 802.11p vehicular communication system, which involves a transmission radius of XX}. 
